# Supplementary material for: Three dimensional waveguide-interconnects for scalable integration of photonic neural networks
Source: arXiv:1912.08203 ancillary file (2020-01-09)
Supplement: Supplementary file 1 [file Suppl-3D_Networks.pdf]

# Supplementary Information for: Three dimensional waveguide-interconnects for scalable integration of photonic neural networks

Johnny Moughames[1], Xavier Porte[1,*], Michael Thiel[2], Gwenn Ulliac[1], Laurent Larger[1], Maxime Jacquot[1], Muamer Kadic[1], and Daniel Brunner[1]

[1]Institut FEMTO-ST, Université Bourgogne Franche-Comté CNRS UMR 6174, Besançon, France.
[2]Nanoscribe GmbH, Hermann-von-Helmholtz-Platz 6, 76344 Eggenstein-Leopoldshafen, Germany
[*]Corresponding author: javier.porte@femto-st.fr

January 9, 2020

## 1 Chiral fractal trees

The branching concept introduced in the main article leverages a fractal, i.e. scale-free approach to link an input channel to a large number of outputs. The number of established connections exponentially grows with the number of bifurcations, and hence this concept efficiently establishes networks with a high degree of connectivity. However, the full interconnect between many IO-channels requires a dedicated coupler for each input channel. As soon as fractal trees of neighboring input channels occupy the same volume, their connections start to intersect, see Fig. S1. The top and bottom rows correspond to projections onto the (x,y) or (x,z) plane, respectively. In each square we introduce the individual units of a 1×9 splitter, plus their arrangement in a 2×2 lattice. The 2×2 arrangement is the smallest network motif where all potential connections, i.e. intersections, are found in the space between the units.

Intersections pose two major challenges. First, they will result in significant crosstalk and additional losses. Second, 3D couplers can at some future stage be amended with phase-shifting elements. This would potentially enable programmable and unitary mapping from the input to the output waveguides, comparable to the 2D Mach-Zehnder meshes [1]. Waveguides intersecting at positions where no interference is desired will almost certainly impede control and programmability.

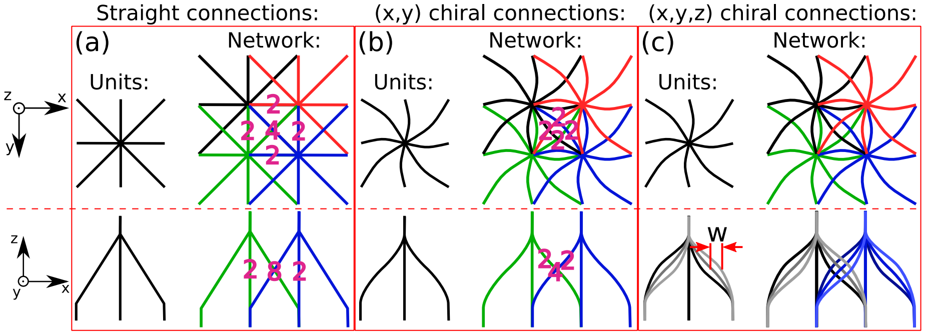


Figure S1: (x,y) and (x,z) projections of fractal trees, with the numbers indicating the amount of intersecting connections at a position. (a) Straight connections results in intersections in horizontal, vertical and diagonal connections. (b) Chirality in the (x,y)-plane eliminates the intersections for horizontal and vertical links. (c) Only for (x,y,z)-chirality all intersections are avoided.

Figure S1(a) illustrates the situation for simply creating a network of 3D fractal couplers with straight connections. The mirror symmetry between neighboring units results in numerous intersecting connections in the space between different couplers (indicated by different colours). Chirality describes the situation when such symmetry is broken, which is what we leverage to avoid intersections.

Between the input of a fractal branching and its output $i$, we have $\Delta x_i$=$x_i^O - x^I$, $\Delta y_i$=$y_i^O$-$y^I$ and $\Delta z_i$=$z_i^O - z^I$ as the distances in $x$, $y$ and $z$, respectively. Superscripts $\{I, O\}$ assign a position to the input and output, respectively. We curve waveguides in the (x,y) plane according to

$$x_i^c(z) = \Delta x_i sin\left[\frac{\pi}{2}\frac{(z - z^I)}{\Delta z_i}\right]^2 \tag{1}$$

$$y_i^c(z) = \Delta y_i sin\left[\frac{\pi}{2}\frac{(z - z^I)}{\Delta z_i}\right]^2, \tag{2}$$

and the resulting structure using $x(z) = x_i^I + x_i^c(z)$ and $y(z) = y_i^I + y_i^c(z)$ is schematically illustrated in Fig. S1(b). Chirality in the (x,y) plane successfully avoids intersections between horizontal and vertical connections.

However, diagonal connections between neighboring trees still appear, though their degeneracy has been reduced: at each point we now simply find two links intersecting. We therefore include chirality also along the z-direction by an

additional displacement in $x$ and $y$

$$x_i^{dz}(z) = w\Delta y_i sin\left[\pi\frac{\sqrt{x_i^c(z)^2 + y_i^c(z)^2}}{\sqrt{\Delta x_i{}^2 + \Delta y_i{}^2}}\right] \tag{3}$$

$$y_i^{dz}(z) = -w\Delta x_i sin\left[\pi\frac{\sqrt{x_i^c(z)^2 + y_i^c(z)^2}}{\sqrt{\Delta x_i{}^2 + \Delta y_i{}^2}}\right], \tag{4}$$

where $w$ is the offset, see Fig. S1(c). Using $x(z) = x_i^I + x_i^c(z) + x_i^{dz}(z)$ and $y(z) = y_i^I + y_i^c(z) + y_i^{dz}(z)$ is schematically illustrated in Fig. S1(c). Here we have used different shading of colors to indicate different positions along the $y$ direction. All crossings are removed, and due to the scale-free nature this approach should be applicable to larger numbers of bifurcation layers.

## 2 Optical Characterization

We have characterized the optical transmission of the 3D-printed polymer waveguides with the experimental setup depicted in Fig. S2. Only optical components are illustrated in this setup. The emission of a semiconductor laser emitting at 635 nm is collimated (Olympus PLN10X) and then focused onto the waveguides' input facets using a 50X microscope objective with NA = 0.8 (Olympus MPLFLN50x). The mode field diameter of the focused beam ($\simeq 2$ $\mu$m) is $\sim 60\%$ larger than the input waveguide's diameter (1.2 $\mu$m). The emission at the waveguides' output ports was collected by a 10X, NA=0.30 microscope objective (Olympus LMPLN10XIR) and imaged onto a CMOS camera (iDS U3-3482LE, pixel size 2.2 $\mu$m) using a 100 mm achromatic lens (Thorlabs AC254-100-B-ML), resulting in an optical magnification of $\simeq 5.6$. A red (635 nm) LED is used as broad field illumination for initial positioning of the sample.

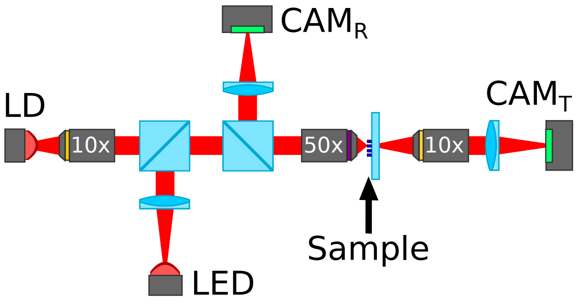


Figure S2: Experimental setup for optical characterization of the 3D printed waveguides. The laser diode (LD) emission was focused onto the top facets of the waveguides by a 50x microscope objective. An LED centered at 635 nm was used as broad field illumination for coarse positioning of the sample. Two CMOS cameras respectively imaged the reflection from the top facet of the waveguides ($CAM_R$) and the transmission through the bottom of the waveguides ($CAM_T$).

The alignment between the focused laser spot and waveguide's input was controlled via imaging the reflection from the top of the waveguide with a second camera ($CAM_R$). The output intensity of the different waveguides was calculated as the integral of an area of $\simeq 4 \times 4\ \mu m^2$ around every waveguide. This area, clearly bigger than the waveguides' input, accounts for inaccuracies determining the centers of the different outputs. By accurately determining the output positions, we can integrate areas 4 times smaller without significant modification of the calculated intensity ratios. Finally, the total transmission losses are calculated after careful calibration of the laser intensity through the sample holder.

# References

[1] D. A. B. Miller, "Perfect optics with imperfect components," Optica **2**, 747 (2015).
